# Supplementary material for: Psychologically-Inspired Causal Prompts
Source: arXiv:2305.01764 source file (2023-05-02)
Supplement: Supplementary file 1 [file sec_additional_analysis.tex]

\subsection{Experimental Details}
The number of parameters of GPT series used in this paper is given in the figure \ref{fig:num_para}. The data is from the document of huggingface and OpenAI.
\begin{figure}[h]
\centering
  \includegraphics[width=0.75\linewidth]{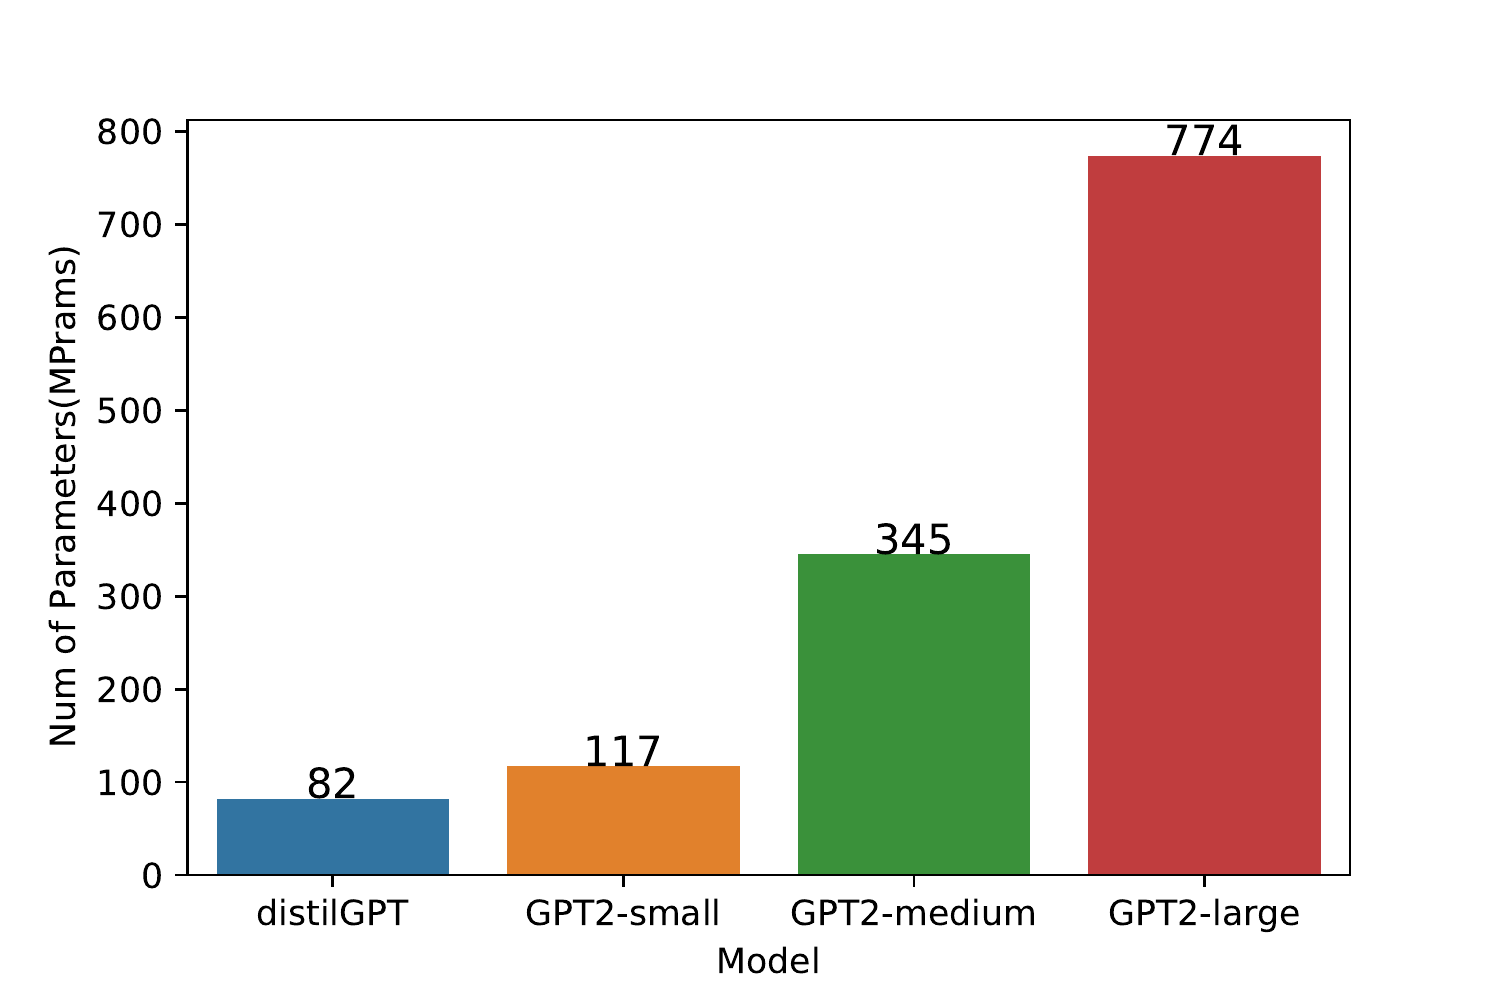}
% \endminipage\hfill
\caption{
    The numbers of parameters of GPT series used in our paper
  }
  \label{fig:num_para}
 \end{figure}

\paragraph{setup of GPT2}
We use the \textsf{transformers} Python library \citep{wolf2019transformers} for GPT2-small, GPT2-medium and GPT2-large. We do not have enough computational resources for GPT2-xl, so we do not test that model. At inference time, we use the defalut Generative Language Model for next token prediction, and use the logits of the tokens ``1,'' ``2,'' ``3,'' ``4,'' and  ``5.''

\paragraph{Implementation Details.}
For the implementation of LLMs, we use the \textsf{transformers} Python library \citep{wolf2019transformers}. Since we do not have enough computational resources for GPT2-xl, we use the second largest GPT2 model, GPT2-large, for our experiment, which is the best autoregressive LLM that we can run and also fits the task (which is more suitable than T5 for this free-form text completion setup). In future work, we will explore more variants of GPTs.
GPT2 series, we use the \textsf{transformers} Python library \citep{wolf2019transformers} for GPT2-small, GPT2-medium and GPT2-large. We do not have enough computational resources for GPT2-xl, so we do not test that model.
For GPT3 series, we use the OpenAI API\footnote{\url{https://openai.com/api}} for GPT3 (using the engine \textsf{davinci}) and InstructGPT (using the engine \textsf{davinci-text-002}). To make our results reproducible, we set the temperature to be 0 for all uses of OpenAI APIs.
For computation efficiency (to save inference time of LLMs), we use some random subsets of the training set, 10K samples to calculate the prior distribution, and another 10K to select the best prompt among a large set of possible paraphrases.

\subsection{Results of All GPTs} 

Our main experimental results are in \cref{tab:res}, where we can see that the true causal prompts (Causal Setup 1) show higher performance than the other ones (Causal Setup 2 \& 3) by a clear margin of 1.9\% by accuracy and 1.94\% by weighted F1. For future work, it will also be interesting to analyze GPTs of different sizes and see if there is a scaling effect of clearer causal distinction as the models get larger.
\begin{table*}[t]
    \centering
    \small
    \begin{tabular}{llccccccc}
    \toprule
       &  & Accuracy & Weighted F1 
    & Accuracy over Paraphrases & Weighted F1 over Paraphrases 
    \\ \midrule
    \multirow{5}{*}{
    Causal Setup 1
    } 
    & GPT3-Instruct & \textbf{69.76 } & \textbf{69.72} & --- & --- \\
    & GPT2-large & 53.71 & 53.68 & \textbf{51.13} & \textbf{51.12}\\
    & GPT2-medium &  34.79 &  31.19 &  35.47 &  32.22\\
    & GPT2-small &  26.98 &  26.68 &  27.05 &  26.90\\
    & distilGPT &  28.18 &  28.19 &  27.83 & 27.64 \\  
    \midrule
    \multirow{5}{*}{Causal Setup 2}
    & GPT3-Instruct & 68.81  & 66.68 & --- & --- \\
    & GPT2-large & 51.81 & 51.74 & 49.41 & 48.93\\
    & GPT2-medium &  32.54 & 32.49 & 32.31 & 31.46\\
    & GPT2-small &  28.05 & 28.02 & 27.74 & 27.40\\
    & distilGPT &  23.65 & 23.67 & 23.38 & 23.17\\ 
    \midrule
    \multirow{5}{*}{Causal Setup 3}
    & GPT3-Instruct & 69.35  & 69.26 & --- & --- \\
    & GPT2-large & 51.84 & 51.77& 49.28 & 48.75 \\
    & GPT2-medium &  41.54 & 40.85 &  41.74 & 40.32\\
    & GPT2-small &  31.17 & 31.15 &  30.75 & 30.47\\
    & distilGPT &  29.41 & 29.40 & 28.95 & 28.71\\
    \bottomrule
    \end{tabular}
    \caption{
    Zero-shot performance of prompts corresponding to all three causal setups on the test set of Yelp. 
    As language models scale to larger sizes, their performance with Setup 1 and Setup 2 are better.
    % Min: one model for all setups and robustness. Better: finish 4 gpt2 models. Even better: improve the setup2 prompt. Best: finish gpt3 davinci models and the other models' performance based on the same test set.
    }
    \label{tab:res}
\end{table*}

\section{Data Subset Features}

% Sentiment Bias is a heuristic metric to reveal the relation between the agreement score and the corpus have more or less positive words than negative, which means the corpus is more likely to be emotional. Due to the frequency of positive words and negative words is different ($\overline{Pos}=6.33$ while $\overline{Neg}=3.12$, we normalized them by divide the frequency in the simple datapoint to the average.

% \paragraph{Sentiment Density}
% $$
% SD = \frac{1}{n}\sum \frac{Pos_i}{\overline{Pos}}+\frac{Neg_i}{\overline{Neg}}
% $$
% Sentiment Density is a heuristic metric to reveal the relation between the agreement score and the corpus have more or less sentiment words, which means the corpus is more likely to be emotional. 

%Here should be the table of the result on GPT3
\paragraph{Overall Explicit Polarity}
Across the entire dataset, we denote the average number of positive words per sample as $\overline{w_{\mathrm{p}}}$, and average number of negative words per sample as $\overline{w_{\mathrm{n}}}$. 

Since a review might have a mixture of positive and negative sentiment words, a rough, simple heuristic is to consider that some opposite sentiments cancel out with each other. Hence, for each sample review $\bm{t}_i \in \bm{D}$, we calculate the difference $|w_{\mathrm{p}}^{i}-w_{\mathrm{n}}^{i}|$ in sentiment words of two different polarities.

Since there is a large difference in the usage frequency of positive and negative words ($\overline{w_{\mathrm{p}}}=6.33$ vs ${\overline{w_{\mathrm{n}}}}=3.12$), we use the difference between the relative frequency of positive words, and that of negative words, namely $\mathrm{OEP} = \sum_{i =0}^K |{w_{\mathrm{p}}^i}/{\overline{w_{\mathrm{p}}}} - {w_{\mathrm{n}}^i}/{\overline{w_{\mathrm{n}}}} |$, for all $K$ samples in a given set.

\section{Related Work}
\paragraph{Design of Prompts}
% 目前很多的工作是关于continuous prompt tuning; prompt training; search discreate prompt in a large space; which is for specific dataset and always biased;performance和dataset具有很强的相关性
% 我们的创新点: 把causal graph embedding进prompt, 然后发现它有用
% XXX讲了在GPTs中构建prompt的一套准则;  我们使用follow的方法构建了prompt 并且由于prompt是脆弱的,我们通过一系列的压力测试证明我们的prompt是local maximum(在prompt空间中相对较好的, 具有代表性的)
%QAQ不知道怎么写了orz 找到的论文应该就以下这些, 本来想说原来的prompt design有各种问题, 所以我们更进一步分析了“让模型理解prompt”这条路的可行性
%说不定可以引一下“let's think step by step”\cite{kojima2022large}

There is a lot of works in design a prompt for a Large Language Model into a specific NLP tasks, ranging from searching the discrete prompt in the prompt space\cite{sorensen2022information}, training the model by  using prompt tokens for a few-shot task\cite{gao2021making} and tuning the co ntinuous prompt\cite{wu2022adversarial,zhu2022continual}. However most of these works just take the prompt learning a alternative of training the whole LLM, but not let the LLM to really understand the meaning of the prompts. Some recent works reveal that short-prompts-based model are biasness \cite{cao2022can}, clueless \cite{kavumba2022prompt} and sensitive \cite{elazar2021measuring}. Our work is more similar to embedding complex information(causal graph) with the prompts and reframing it by some principles \cite{khashabi2022reframing} to find the smallest available prompts containing the correspondent causal graph. The reason for our designing prompt methodology is that we want to minimize the impact of Confounders on our analysis, such as task-irrelevant information in Prompt and linguistic coherence of prompt itself.
%感觉Confounders都是harm performance的会更好说, 就是因为它们是harm的,所以我们尝试去掉所有的Confounders
%然后后面讲我们的prompt的设计过程, 大概可以认为丢进3.1里面
